# Supplementary material for: Multi-reference quantum chemistry protocol for simulating autoionization spectra: Test of ionization continuum models for the neon atom
Source: arXiv:1905.05785 source file (2019-08-27)
Supplement: Supplementary file 1 [file supplement.pdf]

# Supplementary material: Multi-reference quantum chemistry protocol for simulating autoionization spectra: Test of ionization continuum models for the neon atom

Gilbert Grell, Oliver Kühn, and Sergey I. Bokarev*

*Institut für Physik, Universität Rostock,*

*Albert-Einstein-Str. 23-24, 18059, Rostock, Germany*

(Dated: August 27, 2019)

## Abstract

In this contribution we present a protocol to evaluate partial and total Auger decay rates combining the restricted active space self-consistent field electronic structure method for the bound part of the spectrum and numerically obtained continuum orbitals in the single-channel scattering theory framework. On top of that, the two-step picture is employed to evaluate the partial rates. The performance of the method is exemplified for the prototypical Auger decay of the neon $1s^{-1}3p$ resonance. Different approximations to obtain the continuum orbitals, the partial rate matrix elements, and the electronic structure of the bound part are tested against theoretical and experimental reference data. It is demonstrated that the partial and total rates are most sensitive to the accuracy of the continuum orbitals. For instance, it is necessary to account for the direct Coulomb potential of the ion for the determination of the continuum wave functions. The Auger energies can be reproduced quite well already with a rather small active space. Finally, perspectives of the application of the proposed protocol to molecular systems are discussed.

* sergey.bokarev@uni-rostock.de

## I. ADDITIONAL DATA

Here we supply data that were not included in the main text. All abbreviations and naming conventions that have been introduced in the main text are used here without further reiteration.

| potential | (b), $l = 0$ | (c), $l = 1$ | (d), $l = 2$ |
|---|---|---|---|
| $V^{\text{free}}$ | $7.46 \times 10^{-6}$ | $1.14 \times 10^{-4}$ | $7.38 \times 10^{-27}$ |
| $-1/r$ | $7.45 \times 10^{-6}$ | $9.34 \times 10^{-5}$ | $1.43 \times 10^{-26}$ |
| $-6/r$ | $2.65 \times 10^{-6}$ | $1.83 \times 10^{-5}$ | $6.39 \times 10^{-27}$ |
| $V_f^{\text{scr}}(r)$ | $4.54 \times 10^{-7}$ | $3.90 \times 10^{-6}$ | $3.40 \times 10^{-26}$ |
| $V_f^{\text{J}}(r)$ | $3.45 \times 10^{-7}$ | $3.38 \times 10^{-6}$ | $3.61 \times 10^{-26}$ |
| $V_f^{\text{JX}}(r)$ | $1.05 \times 10^{-8}$ | $7.64 \times 10^{-7}$ | $3.79 \times 10^{-26}$ |

TABLE S1. Representative absolute values of continuum-bound overlap integrals for the peaks (b)-(d) from Fig. 3 of the main text. The data has been evaluated using QC scheme I. Shown are the overlap of the continuum orbitals corresponding to the indicated potentials and $l$ quantum numbers with the Dyson orbitals for the respective transition. They have been evaluated as: $\sum_{m=-l}^{l} |\langle\psi_\alpha|\Phi_{i\alpha}\rangle|$; note that compound index $\alpha$ contains $m$ in it. The summation over the spin projections has been dropped for clarity.

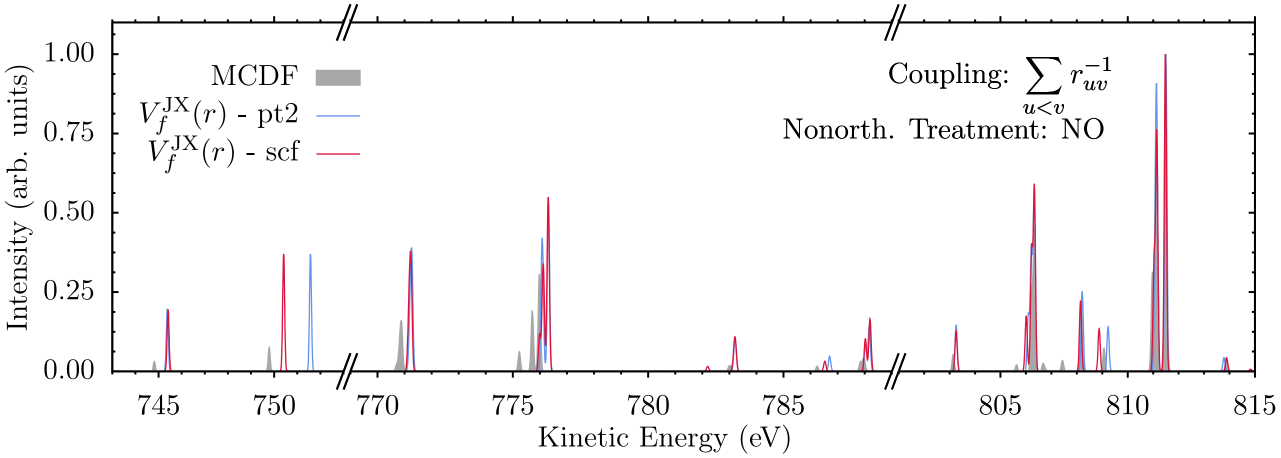


FIG. S1. Comparison of the $r^{-1} \cdot V_f^{JX}(r) \cdot$ NO spectra evaluated using QC scheme I with the RASPT2 correction (pt2) and using the uncorrected RASSCF energies (scf). For reference the MCDF spectrum is shown as well. All spectra are broadened using a Gaussian with an FWHM of 0.1 eV, normalized to the peak at 811.5 eV and shifted globally by −5.35 eV (pt2), −6.75 eV (scf), and −2.45 eV (MCDF).

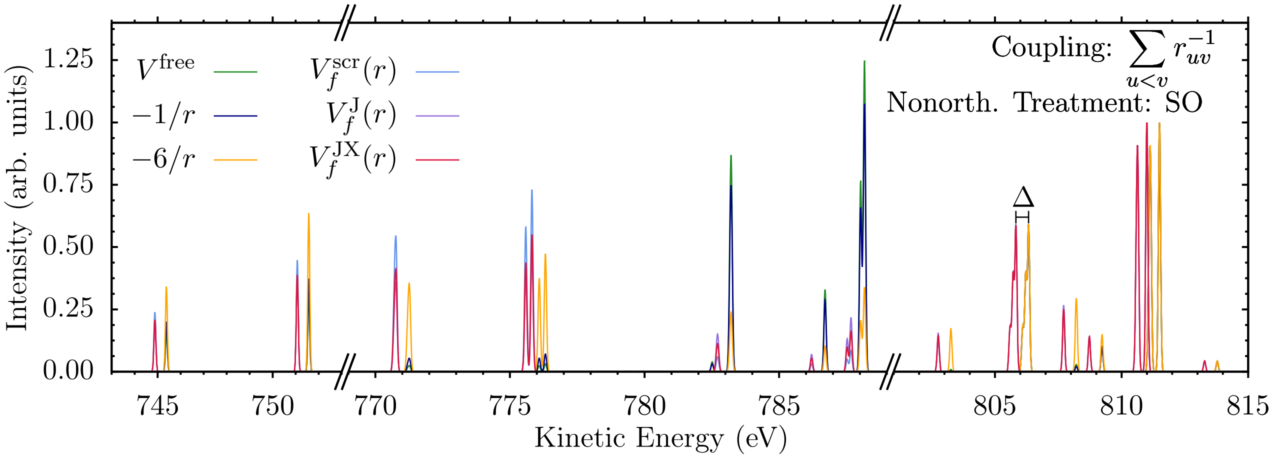


FIG. S2. Spectra obtained for the depicted potentials, using QC scheme I, $r^{-1}$ coupling and the SO approximation. All spectra are broadened using a Gaussian with an FWHM of 0.1 eV, normalized to the peak at 811.5 eV and shifted globally by $-5.35$ eV. For clarity, the spectra obtained with the potentials $V_f^{\mathrm{scr}}(r)$, $V_f^{\mathrm{J}}(r)$ , and $V_f^{\mathrm{JX}}(r)$ have been shifted additionally by $\Delta = -0.5$ eV with respect to the data corresponding to $V^{\mathrm{free}}$, $-1/r$, and $-6/r$.

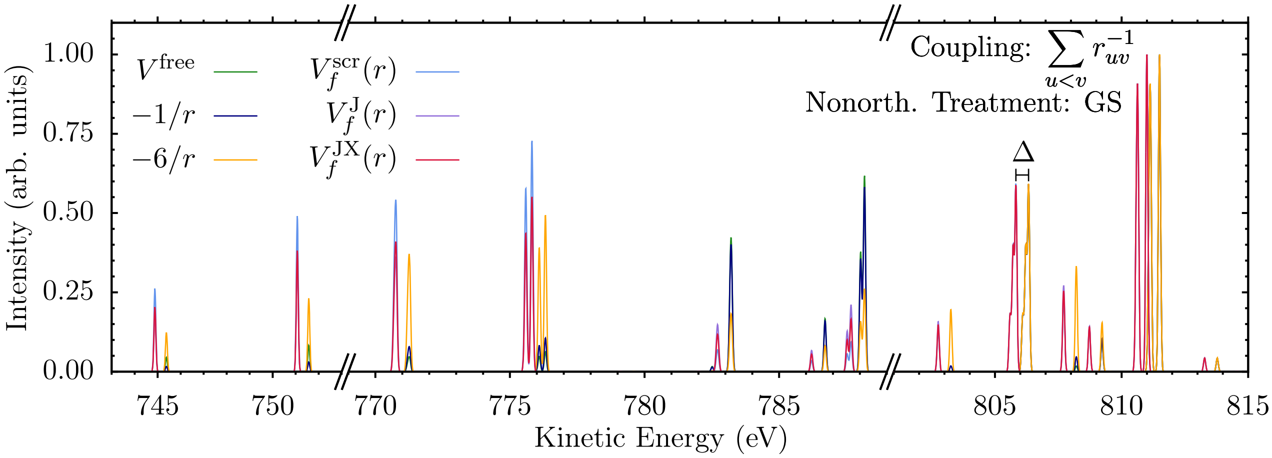


FIG. S3. Spectra obtained for the depicted potentials, using QC scheme I, $r^{-1}$ coupling and the GS approach. All spectra are broadened using a Gaussian with an FWHM of 0.1 eV, normalized to the peak at 811.5 eV and shifted globally by $-5.35$ eV. For clarity, the spectra obtained with the potentials $V_f^{\mathrm{scr}}(r)$, $V_f^{\mathrm{J}}(r)$ , and $V_f^{\mathrm{JX}}(r)$ have been shifted additionally by $\Delta = -0.5$ eV with respect to the data corresponding to $V^{\mathrm{free}}$, $-1/r$, and $-6/r$.

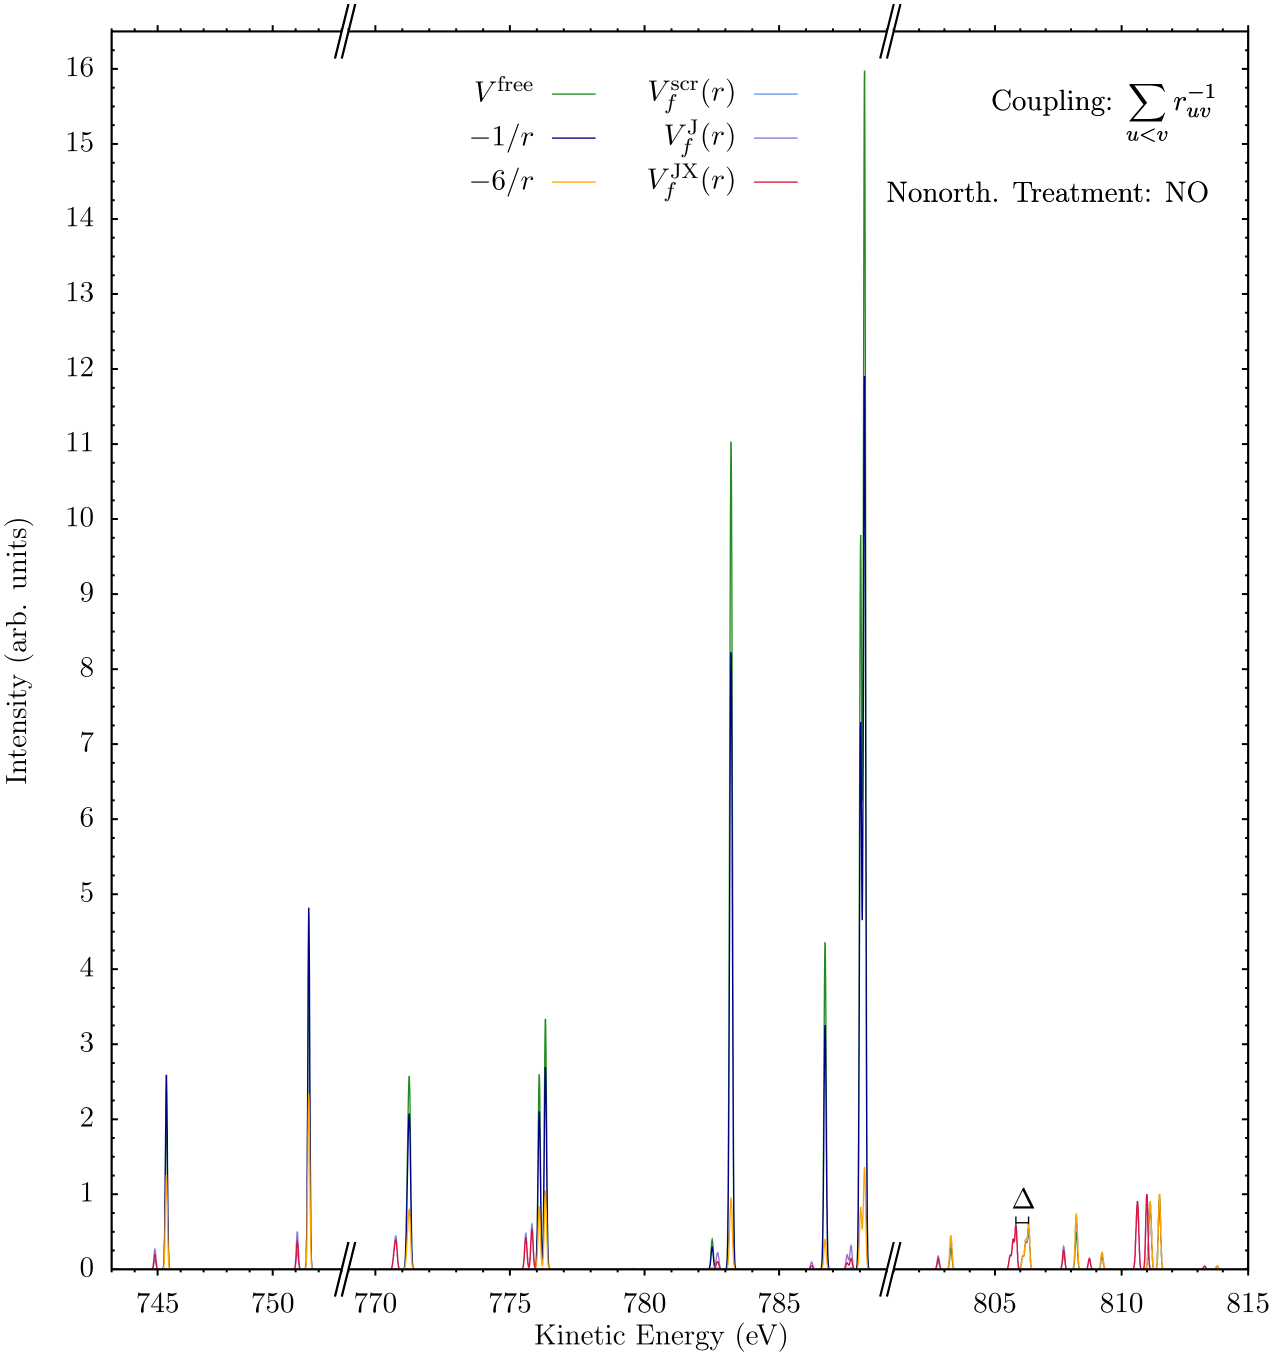


FIG. S4. Spectra obtained for the depicted potentials, using QC scheme I, $r^{-1}$ coupling and the NO approach. All spectra are broadened using a Gaussian with an FWHM of 0.1 eV, normalized to the peak at 811.5 eV and shifted globally by $-5.35$ eV. For clarity, the spectra obtained with the potentials $V_f^{\text{scr}}(r)$, $V_f^{\text{J}}(r)$ , and $V_f^{\text{JX}}(r)$ have been shifted additionally by $\Delta = -0.5$ eV with respect to the data corresponding to $V^{\text{free}}$, $-1/r$, and $-6/r$.

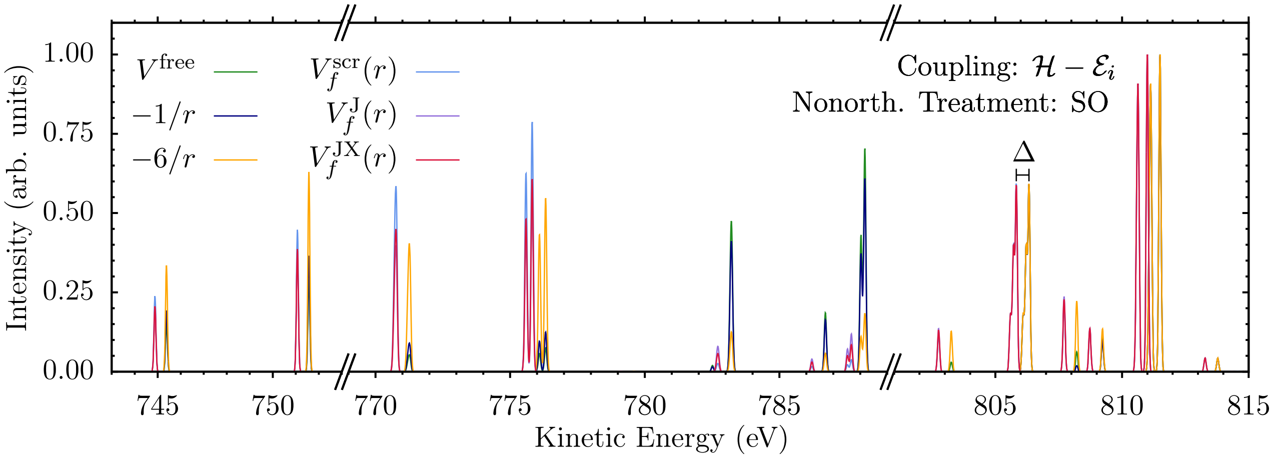


FIG. S5. Spectra obtained for the depicted potentials, using QC scheme I, $\mathcal{H}$ coupling and the SO approximation. All spectra are broadened using a Gaussian with an FWHM of 0.1 eV, normalized to the peak at 811.5 eV and shifted globally by −5.35 eV. For clarity, the spectra obtained with the potentials $V_f^{\text{scr}}(r)$, $V_f^{\text{J}}(r)$ , and $V_f^{\text{JX}}(r)$ have been shifted additionally by $\Delta = -0.5$ eV with respect to the data corresponding to $V^{\text{free}}$, $-1/r$, and $-6/r$.

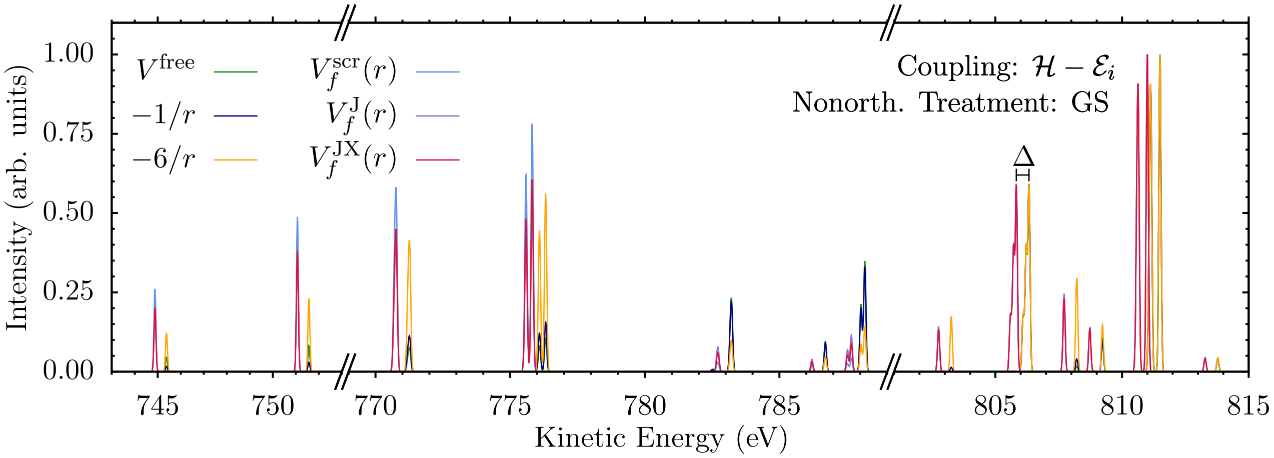


FIG. S6. Spectra obtained for the depicted potentials, using QC scheme I, $\mathcal{H}$ coupling and the GS approach. All spectra are broadened using a Gaussian with an FWHM of 0.1 eV, normalized to the peak at 811.5 eV and shifted globally by −5.35 eV. For clarity, the spectra obtained with the potentials $V_f^{\text{scr}}(r)$, $V_f^{\text{J}}(r)$ , and $V_f^{\text{JX}}(r)$ have been shifted additionally by $\Delta = -0.5$ eV with respect to the data corresponding to $V^{\text{free}}$, $-1/r$, and $-6/r$.

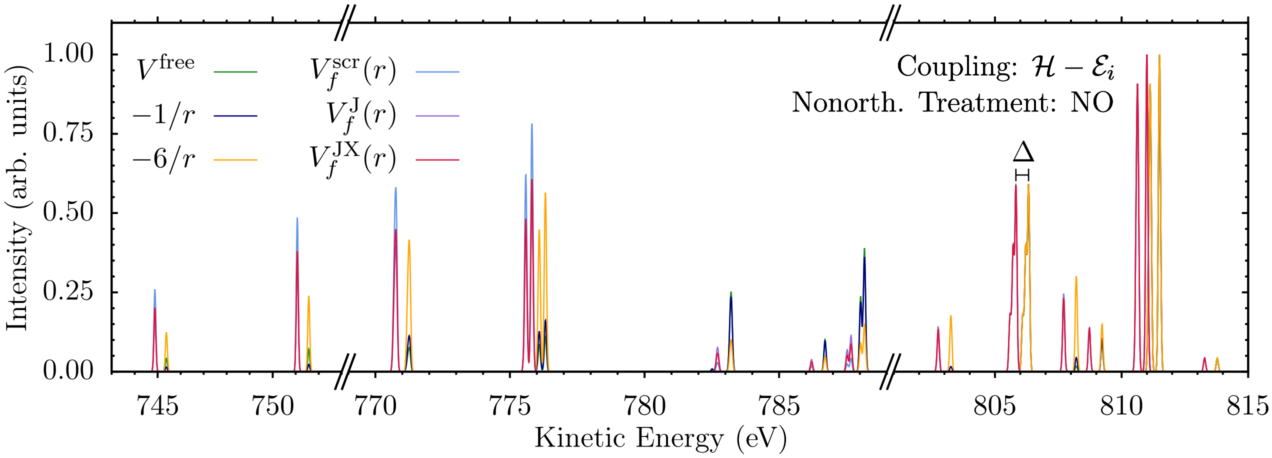


FIG. S7. Spectra obtained for the depicted potentials, using QC scheme I, $\mathcal{H}$ coupling and the NO approach. All spectra are broadened using a Gaussian with an FWHM of 0.1 eV, normalized to the peak at 811.5 eV and shifted globally by −5.35 eV. For clarity, the spectra obtained with the potentials $V_f^{\mathrm{scr}}(r)$, $V_f^{\mathrm{J}}(r)$ , and $V_f^{\mathrm{JX}}(r)$ have been shifted additionally by $\Delta = -0.5$ eV with respect to the data corresponding to $V^{\mathrm{free}}$, $-1/r$, and $-6/r$.

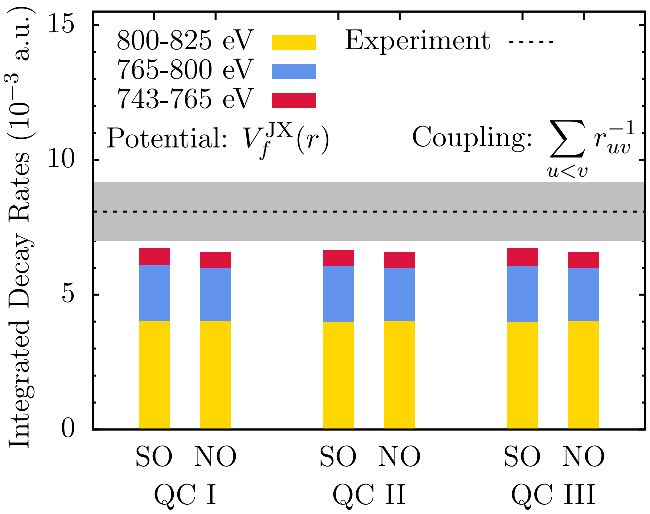


FIG. S8. Comparison of the neon $1s^{-1}3p$ Auger decay rates integrated over the given spectral regions. The partial rates have been obtained based on the QC schemes I,II and III using the $r^{-1}$ coupling, the $V_f^{JX}(r)$ potential, and either of the NO or SO nonorthogonality approaches. For reference, the experimental ($8.08 \pm 1.1 \times 10^{-3}$ a.u. [1]) value of the total Auger decay rate is given.

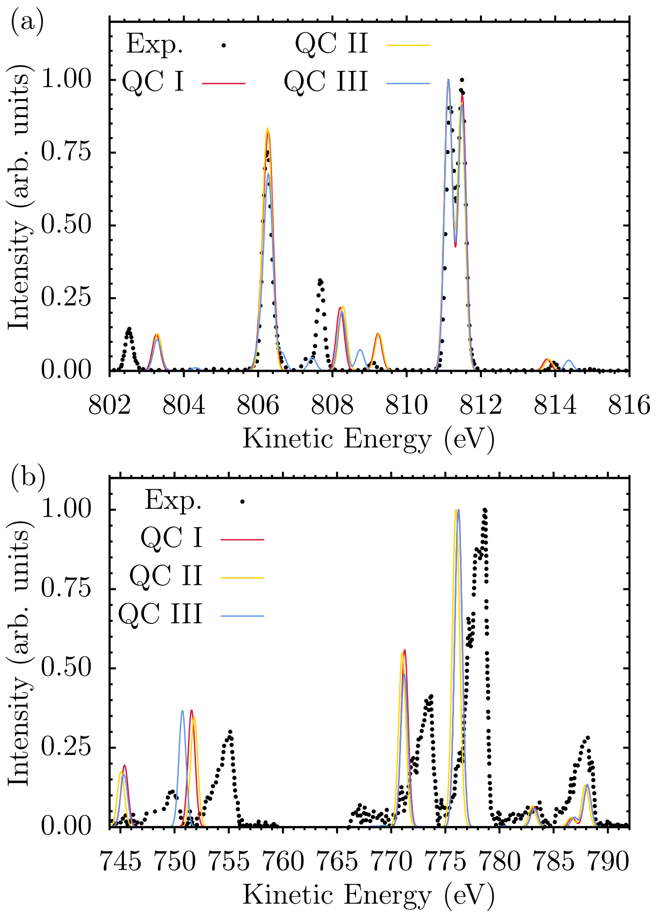


FIG. S9. Comparison of experimental and theoretical neon $1s^{-1}3p$ AES obtained based on the QC schemes I - III with the $\mathcal{H} \cdot V_f^{\mathrm{JX}}(r) \cdot \mathrm{NO}$ method. The spectra obtained with QC I, II, and III have been shifted by $-5.35$ eV, $-4.75$ eV, and $-5.18$ eV, respectively, to align the peak at 811.5 eV with the experimental data in panel (a). To account for the different lineshapes of the experimental spectra that have been digitalized from [2], panel (a), and [3] in panel (b), broadening with a Gaussian FWHM of 0.25 eV and 0.77 eV was used in panels (a) and (b), respectively. Further, the spectra have been normalized individually to the peaks at 811.5 eV (a) and 776 eV (b).

## II. THE EVALUATION OF THE NO CORRECTION TERMS

In Ref. 4, Manne and Ågren have described a general way to compute the Auger transition matrix elements, based only on the fundamental assumption that the involved wave functions can be written as linear combinations of Slater determinants, that are in turn constructed out of a set of orthonormal orbitals. In brief, using the same notation as in the main text their results can be summarized as follows:

We start with the continuum state $|\Psi_\alpha\rangle$ being decomposed into the channel functions: $|\Psi_\alpha\rangle = \sum_{M^+=-S^+}^{S^+} \sum_{\sigma=-\frac{1}{2},\frac{1}{2}} C_{S^+,M^+;\sigma}^{S,M} \left|\Upsilon_\alpha^{M^+,\sigma}\right\rangle$. These are defined by acting with the creation operator of the continuum orbital on the corresponding bound state of the ionized system, $\left|\Upsilon_\alpha^{\sigma M^+}\right\rangle = a_{\alpha,\sigma}^\dagger \left|\Psi_{f,M^+}^+\right\rangle$ . We shall not discuss the summation of different spins here and thus drop the spin indices completely in what follows. The Auger matrix element for one channel function may then be expressed as :

$$A_{i\alpha} = \left\langle\Psi_f^+\middle|a_\alpha(\mathcal{H}-\mathcal{E}_i)\middle|\Psi_i\right\rangle \tag{S1}$$

Employing the commutator $[a_\alpha, \mathcal{H}]$ Manne and Åberg proceed to express the matrix element as

$$A_{i\alpha} = \left\langle\Psi_f^+\middle|[a_\alpha,\mathcal{H}]\middle|\Psi_i\right\rangle + \left\langle\Psi_f^+\middle|(\mathcal{H}-\mathcal{E}_i)a_\alpha\middle|\Psi_i\right\rangle \tag{S2}$$

Now, they suppose that $\left\langle\Psi_f^+\right|$ is indeed an eigenstate of the Hamiltonian and exploit the eigenvalue equation $\left\langle\Psi_f^+\right|\mathcal{H} = \left\langle\Psi_f^+\right|\mathcal{E}_f$ together with the definition of the energy of the ionized electron $\varepsilon_\alpha = \mathcal{E}_i - \mathcal{E}_f$, which gives:

$$A_{i\alpha} = \left\langle\Psi_f^+\middle|[a_\alpha,\mathcal{H}]\middle|\Psi_i\right\rangle - \varepsilon_\alpha\left\langle\Psi_f^+\middle|a_\alpha\middle|\Psi_i\right\rangle \tag{S3}$$

To obtain an practically useful equation, the Hamiltonian and annihilation operator need to be expressed in the basis of the ionized and unionized states: These basis functions are the spin orbitals $\{\varphi_s\}$ and $\{\varphi_q^+\}$ corresponding to $|\Psi_i\rangle$ and $\left|\Psi_f^+\right\rangle$. In the RASSCF family of methods, these are defined as the eigenfunctions of effective Fockians $\mathcal{F}$ and $\mathcal{F}^+$,

corresponding to the unionized and ionized states:

$$\mathcal{F}\left|\varphi_s\right\rangle = \varepsilon_s \left|\varphi_s\right\rangle, \tag{S4}$$

$$\mathcal{F}^+\left|\varphi_q^+\right\rangle = \varepsilon_q^+ \left|\varphi_q^+\right\rangle. \tag{S5}$$

To continue, one has to assume that the Fockians are constructed from a complete basis, and that their spectrum of eigenfunctions and eigenvalues comprises a bound and a continuous part. Given this, the annihilator may be expressed in the basis corresponding to the unionized state as:

$$a_\alpha = \sum_s \left\langle \psi_\alpha | \varphi_s \right\rangle a_s + \int \left\langle \psi_\alpha | \varphi(\beta) \right\rangle a(\beta) d\beta = \sum\!\!\!\!\!\!\int \left\langle \psi_\alpha | \varphi(s) \right\rangle a(s) ds\,. \tag{S6}$$

Where the greek and latin indices indicate the continuous and discrete part of the spectrum of $\mathcal{F}$. As a compromise, the abbreviated sum + integral notation employs the latin index in a functional dependence. Note that the discrete and continuous eigenfunctions can always be clearly distinguished, because the former are square integrable function, while the latter are not, i.e. they fulfill the normalization relation:

$$\left\langle \varphi(r) | \varphi(s) \right\rangle = \delta(r,s) = \begin{cases} \delta_{rs} & \text{discrete spectrum} \\ \delta(\varepsilon_r - \varepsilon_s) & \text{continuous spectrum} \end{cases} \tag{S7}$$

Since both basis are complete and can be converted into each other, it is convenient to express the Hamiltonian by using the the basis $\{\varphi_i^+\}$ and $\{\varphi_i\}$ for the creation and annihilation operators, respectively:

$$\mathcal{H} = \sum\!\!\!\!\!\!\int \mathrm{d}q \mathrm{d}s\, h_1(q,s) \left(a^+(q)\right)^\dagger a(s) \tag{S8}$$

$$+ \frac{1}{2} \sum\!\!\!\!\!\!\int \mathrm{d}q_1 \mathrm{d}q_2 \mathrm{d}s_1 \mathrm{d}s_2\, h_2(q_1,q_2;s_1,s_2) \left(a^+(q_1)\right)^\dagger \left(a^+(q_2)\right)^\dagger a(s_2) a(s_1) \tag{S9}$$

Where the operators act as $(a^+(q))^\dagger \left|0\right\rangle = \left|\varphi^+(q)\right\rangle$ and $a^\dagger(s)\left|0\right\rangle = \left|\varphi(s)\right\rangle$, and

$$h_1(q,s) = \left\langle \varphi^+(q) \middle| h \middle| \varphi(s) \right\rangle \tag{S10}$$

$$h_2(q_1,q_2;s_1,s_2) = \left\langle \varphi^+(q_1)\varphi^+(q_2) \middle| \varphi(s_1)\varphi(s_2) \right\rangle \tag{S11}$$

Using the anticommutators

$$[a_\alpha, \left(a^+(q)\right)^\dagger]_+ = \left\langle \psi_\alpha \middle| \varphi^+(q) \right\rangle, \tag{S12}$$

$$[a_\alpha, a(q)]_+ = 0, \tag{S13}$$

$$[a(t), a(s)]_+ = 0, \tag{S14}$$

and Eq. (S8), the matrix element involving the commutator in Eq. (S3) can be expressed as:

$$\begin{aligned}\left\langle \Psi_f^+ \middle| [a_\alpha, \mathcal{H}] \middle| \Psi_i \right\rangle = &\sum\!\!\!\!\!\!\int \mathrm{d}s\, h_1(\alpha, s) \left\langle \Psi_f^+ \middle| a(s) \middle| \Psi_i \right\rangle \\ &+ \sum\!\!\!\!\!\!\int \mathrm{d}q \mathrm{d}s_1 \mathrm{d}s_2 h_2(\alpha, q; s_1, s_2) \left\langle \Psi_f^+ \middle| \left(a^+(q)\right)^\dagger a(s_2) a(s_1) \middle| \Psi_i \right\rangle\end{aligned} \tag{S15}$$

Finally, one uses the fact that by definition the states $|\Psi_i\rangle$ and $\left|\Psi_f^+\right\rangle$ are purely bound states. Consequently, any continuum annihilation operator applied to these states produces zeros, i.e. $a(s)\,|\Psi_i\rangle = 0$ and $\left\langle \Psi_f^+ \right| a_+(q)^\dagger = 0$, if the operators correspond to the continuum. This allows to disregard the continuum integration in Eq. (S15) and to express the full matrix element as

$$\begin{aligned}A_{i\alpha} = &\sum_s^{N_\mathrm{orb}} \langle \psi_\alpha | h | \varphi_s \rangle \left\langle \Psi_f^+ \middle| a_s \middle| \Psi_i \right\rangle + \sum_q^{N_\mathrm{orb}} \sum_{s_1 \neq s_2}^{N_\mathrm{orb}} \left\langle \psi_\alpha \varphi_q^+ \middle| \varphi_{s_1} \varphi_{s_2} \right\rangle \left\langle \Psi_f^+ \middle| (a_q^+)^\dagger a_{s_2} a_{s_1} \middle| \Psi_i \right\rangle \\ &- \varepsilon_\alpha \sum_s^{N_\mathrm{orb}} \left\langle \Psi_f^+ \middle| a_s \middle| \Psi_i \right\rangle \langle \psi_\alpha | \varphi_s \rangle ,\end{aligned} \tag{S16}$$

where we have used the expansion (S6), again reduced to the discrete part. This is the celebrated result of Manne and Åberg [4]. Using the definitions for the Dyson orbital $|\Phi_{i\alpha}\rangle$ and the two-electron reduced transition density $|\Xi_{i\alpha}^q\rangle$ in Eqs. (15) and (18), the matrix element takes the form:

$$A_{i\alpha} = \langle \psi_\alpha | h | \Phi_{i\alpha} \rangle + \sum_q^{N_\mathrm{orb}} \left\langle \psi_\alpha \varphi_q^+ \middle| \frac{1}{r_{12}} \middle| \Xi_{i\alpha}^q \right\rangle - \varepsilon_\alpha \langle \psi_\alpha | \Phi_{i\alpha} \rangle . \tag{S17}$$

While this formulation is straightforwardly derived, subtle problems are encountered in the actual evaluation of the term that arises due to the nonorthogonality of the continuum

and bound orbitals of the unionized system, i.e. the NO term $\varepsilon_\alpha \langle\psi_\alpha|\Phi_{i\alpha}\rangle$. In our implementation, we derived all matrix elements in first quantization using Löwdin's calculus for transition matrix elements between Slater determinants in a nonorthogoanl basis [5]. Naturally, this formalism cannot make use of elegant simplifications by using the commutation relations as in Eq. (S3) to reexpress the matrix elements. However, one can of course relate the determinant based first quantized formalism to the second quantized one as was done in the Theory section of this paper. It is possible to rearrange the NO-terms in such a way that a relation similiar to the second term in Eq. (S3) is obtained, namely:

$$A_{i\alpha}^{\mathrm{NO}} = \sum_{t}^{N_{\mathrm{orb}}^{\mathrm{occ}}} \langle\psi_\alpha|\varphi_t\rangle \tag{S18}$$

$$\times \left\langle\Psi_f^+\right|\Bigg(\underbrace{\sum_{q,s}^{N_{\mathrm{orb}}^{\mathrm{occ}}} \left\langle\varphi_q^+\middle|h\middle|\varphi_s\right\rangle (a_q^+)^\dagger a_s + \frac{1}{2}\sum_{\substack{q_1\neq q_2\\ s_1\neq s_2}}^{N_{\mathrm{orb}}^{\mathrm{occ}}} \left\langle\varphi_{q_1}^+\varphi_{q_2}^+\middle|\frac{1}{r_{12}}\middle|\varphi_{s_2}\varphi_{s_1}\right\rangle (a_{q_1}^+)^\dagger(a_{q_2}^+)^\dagger a_{s_2}a_{s_1} - \mathcal{E}_i}_{\tilde{\mathcal{H}}}\Bigg) a_t\left|\Psi_i\right\rangle \tag{S19}$$

Note that two first sums in the parentheses correspond to Hamiltonian matrix $\tilde{\mathcal{H}}$ in the mixed basis. Here, the limit $N_{\mathrm{orb}}^{\mathrm{occ}}$ indicates that the summation is carried out only over orbitals $\varphi_s$, $\varphi_q^+$ that may be occupied in the states $|\Psi_i\rangle$ and $\left|\Psi_f^+\right\rangle$, respectively. That is inactive and active ones within RASSCF formalism. To show the equivalence, i.e. that $A_{i\alpha}^{\mathrm{NO}} = \left\langle\Psi_f^+\middle|(\mathcal{H}-\mathcal{E}_i)a_\alpha\middle|\Psi_i\right\rangle$, we need first to transform the Hamiltonian $\tilde{\mathcal{H}}$ to the basis of the ionized state $\left|\Psi_f^+\right\rangle$. This is achieved by expanding the annihilation operators $a_s$ in the ionized basis:

$$a_s = \sum_{q}^{N_{\mathrm{orb}}} \left\langle\varphi_s\middle|\varphi_q^+\right\rangle a_q^+ \tag{S20}$$

Here, however, one has to take into account all, i.e. occupied and virtual orbitals: $N_{\mathrm{orb}} = N_{\mathrm{orb}}^{\mathrm{occ}} + N_{\mathrm{orb}}^{\mathrm{virt}}$. Second, the ket orbitals need to be contracted with the the overlap integrals using the completeness:

$$\left|\varphi_q^+\right\rangle = \sum_{s}^{N_{\mathrm{orb}}} \left\langle\varphi_s\middle|\varphi_q^+\right\rangle |\varphi_s\rangle \tag{S21}$$

In Eq. (S18), however, the summation spans only the space of the occupied unionized orbitals $\varphi_s$. Hence we can in generally not transform the operator $\tilde{\mathcal{H}}$ into a proper Hamiltonian

$$\mathcal{H}^+ = \sum_{q_1,q_2}^{N_{\rm orb}^{\rm occ}} \langle \varphi_{q_1}^+ | h | \varphi_{q_2}^+ \rangle \, (a_{q_1}^+)^\dagger a_{q_2}^+ + \frac{1}{2} \sum_{\substack{q_1 \neq q_2 \\ q_3 \neq q_4}}^{N_{\rm orb}^{\rm occ}} \langle \varphi_{q_1}^+ \varphi_{q_2}^+ | \frac{1}{r_{12}} | \varphi_{q_3}^+ \varphi_{q_4}^+ \rangle \, (a_{q_1}^+)^\dagger (a_{q_2}^+)^\dagger a_{q_4}^+ a_{q_3}^+ \tag{S22}$$

that allows the exploitation of $\mathcal{H}^+ \left| \Psi_f^+ \right\rangle = \mathcal{E}_f \left| \Psi_f^+ \right\rangle$. The only exceptions to this rule are cases, when the occupied orbitals used for the ionized and unionized states span the same Hilbert space. Two particular cases, where this is true are Full-CI calculations and calculations in frozen orbital approximation, where the ionized wave functions are obtained using the unionized orbital basis, or vice-versa.

In brief this can by summarized in the following statements: Due to the fact that the wave functions for the bound ionized and unionized states are obtained in independent RASSCF calculations, these wave functions generally belong to different Hilbert spaces. A consequence of this is that the NO terms evaluated using the second quantization approach of Manne and Åberg [4], exploiting the eigenvalue equation $\mathcal{H} \left| \Psi_f^+ \right\rangle = \mathcal{E}_f \left| \Psi_f^+ \right\rangle$, deviate from the ones evaluated using the approach presented in the main text in Eqs. (12)-(18). These two approaches give equal results only, if wave functions actually span the same space, e.g., in full CI approach or using the frozen orbital approximation. Further, the eigenvalue equation can in principle only be used, if the coupling Hamiltonian is the same as the one used in the wave function optimization. This regards especially perturbative energetic corrections, or the inclusion of scalar relativistic effects, which are often included in the SCF procedures, but in our case not in the evaluation of the coupling matrix element. For the decay of the neon $1s^{-1}3p$ resonance, evaluated using QC scheme I with and without RASPT2 corrected energies, the difference between both approaches is indicated in Fig. S10. The integrated decay rates evaluated using the RASPT2 corrected and the original RASSCF state energies, do not visibly differ, indicating, that the pt2 terms can in this case be neglected from the coupling Hamiltonian.

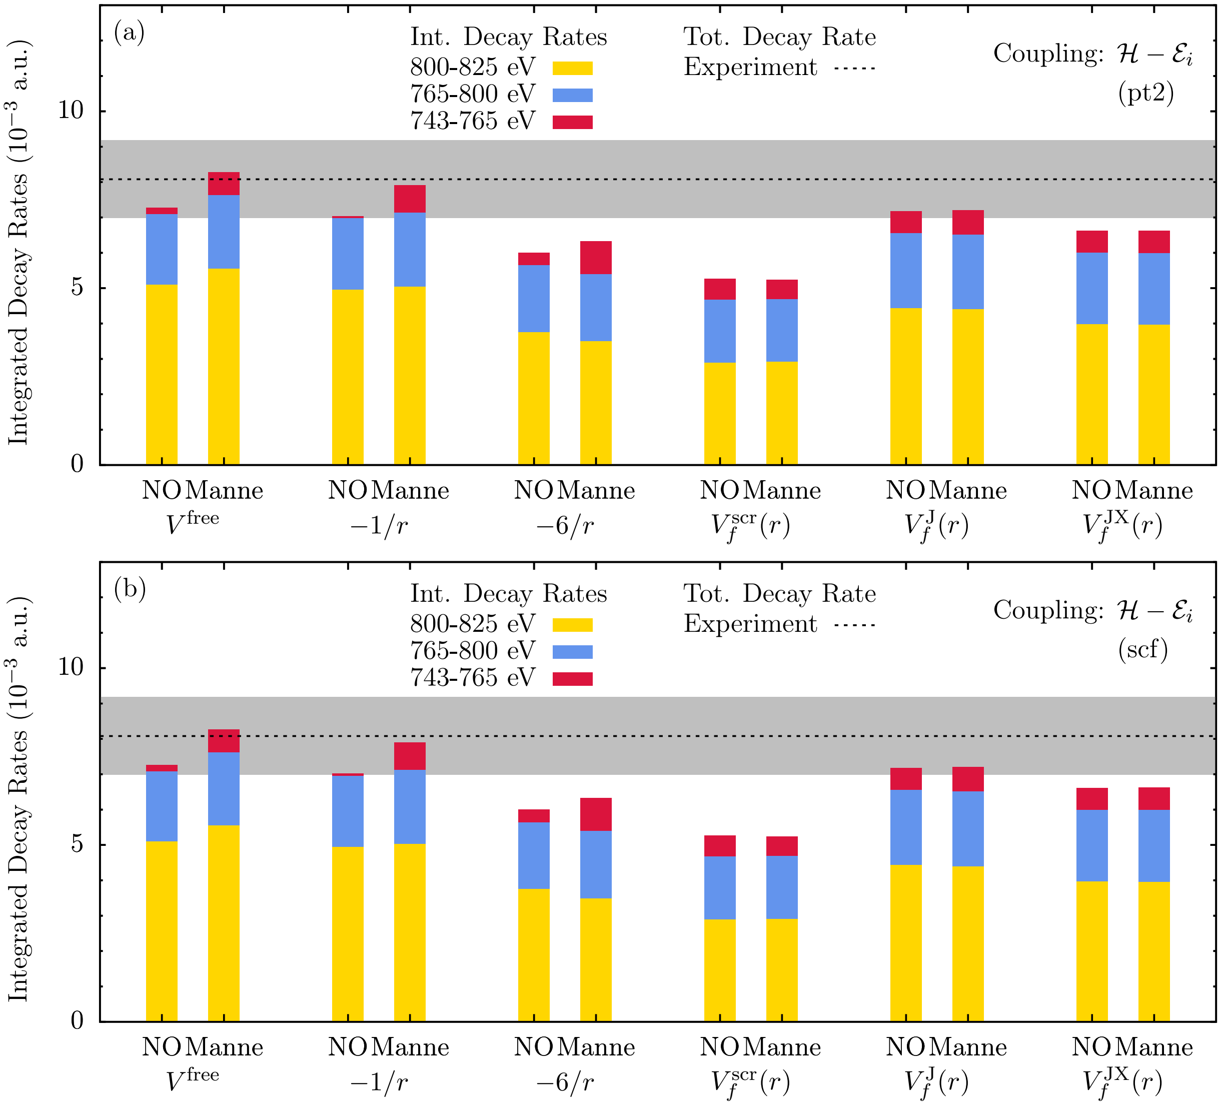


FIG. S10. Comparison of the neon $1s^{-1}3p$ Auger decay rates integrated over the given spectral regions. Data in(a) and (b) were obtained using the underlying QC scheme I, with and without the RASPT2 correction. The partial rates have been obtained using the $\mathcal{H}$ coupling, all potential models and either the NO approach as discussed in the main text of the paper and in Eq. (S18) (NO), or the one suggested in Ref. 4, corresponding to Eq. (S3) (Manne). For reference, the experimental ($8.08 \pm 1.1 \times 10^{-3}$ a.u. [1]) value of the total Auger decay rate is given.

## III. BASIS SETS

- QC I: (22s17p12d11f)/[7s6p3d2f]

```
 Ne S
166165.08     0.0000  -0.0000   0.0000  -0.0000   0.0000  -0.0000   0.0000
23107.524     0.0004  -0.0001   0.0000  -0.0000   0.0000  -0.0000   0.0000
5060.1539     0.0022  -0.0005   0.0001  -0.0000   0.0000  -0.0001   0.0001
1384.6123     0.0096  -0.0024   0.0004  -0.0001   0.0000  -0.0004   0.0004
436.51258     0.0351  -0.0089   0.0015  -0.0004   0.0001  -0.0015   0.0016
153.47148     0.1049  -0.0277   0.0046  -0.0012   0.0002  -0.0047   0.0049
59.389087     0.2385  -0.0693   0.0117  -0.0031   0.0006  -0.0120   0.0124
24.861967     0.3704  -0.1311   0.0220  -0.0057   0.0012  -0.0222   0.0230
11.015704     0.3054  -0.1662   0.0309  -0.0082   0.0017  -0.0325   0.0341
4.9651750     0.0832  -0.0071   0.0015  -0.0002   0.0000  -0.0008   0.0021
1.9365030     0.0033   0.4415  -0.0849   0.0220  -0.0045   0.0894  -0.0982
0.76572800    0.0007   0.5713  -0.1913   0.0547  -0.0118   0.2388  -0.2584
0.29553800   -0.0001   0.1218  -0.1230   0.0394  -0.0132   0.1114  -0.0841
0.10343800    0.0002  -0.0130   0.1017  -0.0460   0.0066  -0.7688   1.0169
0.06564559   -0.0002   0.0089   0.3612  -0.1964   0.0610  -0.8099   0.6778
0.02462393    0.0001  -0.0035   1.2334  -0.8336   0.8883   1.8774  -3.0894
0.01125334   -0.0001   0.0036  -0.6690   0.9454  -1.8079  -0.0414   1.6952
0.00585838    0.0002  -0.0040  -0.5411   0.9891  -1.3819  -0.9776   3.4980
0.00334597   -0.0002   0.0044   0.6793  -0.4056   2.9154   0.1501  -5.6430
0.00204842    0.0002  -0.0041  -0.0644   0.1257  -0.3728  -1.7904   1.0781
0.00132364   -0.0001   0.0023   0.0417  -0.0656   0.2021   2.0906   0.9034
0.00089310    0.0000  -0.0006  -0.0258   0.0241  -0.1583   0.1710   0.6692
Ne P
234.94500     0.0018  -0.0002   0.0000  -0.0000   0.0004  -0.0003
55.077385     0.0143  -0.0017   0.0001  -0.0003   0.0028  -0.0026
17.389549     0.0653  -0.0081   0.0004  -0.0015   0.0129  -0.0121
6.3895370     0.1918  -0.0246   0.0011  -0.0045   0.0398  -0.0377
2.5420820     0.3494  -0.0492   0.0022  -0.0091   0.0823  -0.0793
1.0337640     0.3958  -0.0562   0.0025  -0.0101   0.0943  -0.0900
0.41878800    0.2048  -0.0311   0.0026  -0.0070   0.0292  -0.0140
0.16462700    0.0139   0.1027  -0.0123   0.0127  -0.3868   0.3837
0.05761900    0.0095   0.2481  -0.0285  -0.0296  -1.3944   1.3447
0.04233528   -0.0113   0.3076  -0.0647   0.2715   1.0749  -1.1970
0.01925421    0.0063   0.8708  -0.1525   0.5566   0.9404  -1.1293
0.00998821   -0.0075  -0.5514   0.4601  -1.5324  -0.4657   0.9914
0.00568936    0.0095  -0.1837   0.4750  -0.6211  -0.2237   1.3645
0.00347568   -0.0102  -0.1157   0.2575   1.2679   0.0567  -2.0164
0.00224206    0.0083   0.2662  -0.0324   0.5138  -0.6760  -0.0023
0.00151064   -0.0047  -0.0682   0.0319   0.2608  -0.1087  -0.6459
0.00105475    0.0013  -0.0217  -0.0090  -0.3426   1.2059   1.6974
Ne D
6.4200000     0.0002  -0.0016   0.0020
2.2470000     0.0007  -0.0046   0.0058
0.78645000    0.0034  -0.0260   0.0340
0.275257500   0.0042  -0.0365   0.0489
0.16329773    0.0195  -0.1902   0.2497
0.06054020    0.0894  -0.5041   0.5975
0.02744569    0.3365  -0.1129  -0.1793
0.01420440    0.4900   0.0937  -0.5889
0.00807659    0.1965   0.1198  -0.1697
0.00492719    0.0129   0.2599   0.4914
0.00317481   -0.0284   0.2720   0.3012
0.00213712   -0.0158   0.1298   0.2098
Ne F
4.1900000     0.0000  -0.0000
1.6760000     0.0001  -0.0002
0.67040000    0.0008  -0.0014
0.21400555    0.0121  -0.0225
0.07906987    0.0892  -0.1611
0.03576293    0.2559  -0.4308
0.01847779    0.3113  -0.3363
0.01049301    0.2119   0.1208
0.00639492    0.2212   0.4092
0.00411721    0.1148   0.2259
0.00276965    0.0981   0.1924
```

- QC II: (22s17p12d11f)/[22s6p3d2f]-rcc

```
Ne S
166165.08     1.0 0.0 0.0 0.0 0.0 0.0 0.0 0.0 0.0 0.0 0.0 0.0 0.0 0.0 0.0 0.0 0.0 0.0 0.0 0.0 0.0 0.0
23107.524     0.0 1.0 0.0 0.0 0.0 0.0 0.0 0.0 0.0 0.0 0.0 0.0 0.0 0.0 0.0 0.0 0.0 0.0 0.0 0.0 0.0 0.0
5060.1539     0.0 0.0 1.0 0.0 0.0 0.0 0.0 0.0 0.0 0.0 0.0 0.0 0.0 0.0 0.0 0.0 0.0 0.0 0.0 0.0 0.0 0.0
1384.6123     0.0 0.0 0.0 1.0 0.0 0.0 0.0 0.0 0.0 0.0 0.0 0.0 0.0 0.0 0.0 0.0 0.0 0.0 0.0 0.0 0.0 0.0
436.51258     0.0 0.0 0.0 0.0 1.0 0.0 0.0 0.0 0.0 0.0 0.0 0.0 0.0 0.0 0.0 0.0 0.0 0.0 0.0 0.0 0.0 0.0
153.47148     0.0 0.0 0.0 0.0 0.0 1.0 0.0 0.0 0.0 0.0 0.0 0.0 0.0 0.0 0.0 0.0 0.0 0.0 0.0 0.0 0.0 0.0
59.389087     0.0 0.0 0.0 0.0 0.0 0.0 1.0 0.0 0.0 0.0 0.0 0.0 0.0 0.0 0.0 0.0 0.0 0.0 0.0 0.0 0.0 0.0
24.861967     0.0 0.0 0.0 0.0 0.0 0.0 0.0 1.0 0.0 0.0 0.0 0.0 0.0 0.0 0.0 0.0 0.0 0.0 0.0 0.0 0.0 0.0
11.015704     0.0 0.0 0.0 0.0 0.0 0.0 0.0 0.0 1.0 0.0 0.0 0.0 0.0 0.0 0.0 0.0 0.0 0.0 0.0 0.0 0.0 0.0
4.9651750     0.0 0.0 0.0 0.0 0.0 0.0 0.0 0.0 0.0 1.0 0.0 0.0 0.0 0.0 0.0 0.0 0.0 0.0 0.0 0.0 0.0 0.0
1.9365030     0.0 0.0 0.0 0.0 0.0 0.0 0.0 0.0 0.0 0.0 1.0 0.0 0.0 0.0 0.0 0.0 0.0 0.0 0.0 0.0 0.0 0.0
0.76572800    0.0 0.0 0.0 0.0 0.0 0.0 0.0 0.0 0.0 0.0 0.0 1.0 0.0 0.0 0.0 0.0 0.0 0.0 0.0 0.0 0.0 0.0
0.29553800    0.0 0.0 0.0 0.0 0.0 0.0 0.0 0.0 0.0 0.0 0.0 0.0 1.0 0.0 0.0 0.0 0.0 0.0 0.0 0.0 0.0 0.0
0.10343800    0.0 0.0 0.0 0.0 0.0 0.0 0.0 0.0 0.0 0.0 0.0 0.0 0.0 1.0 0.0 0.0 0.0 0.0 0.0 0.0 0.0 0.0
0.06564559    0.0 0.0 0.0 0.0 0.0 0.0 0.0 0.0 0.0 0.0 0.0 0.0 0.0 0.0 1.0 0.0 0.0 0.0 0.0 0.0 0.0 0.0
0.02462393    0.0 0.0 0.0 0.0 0.0 0.0 0.0 0.0 0.0 0.0 0.0 0.0 0.0 0.0 0.0 1.0 0.0 0.0 0.0 0.0 0.0 0.0
0.01125334    0.0 0.0 0.0 0.0 0.0 0.0 0.0 0.0 0.0 0.0 0.0 0.0 0.0 0.0 0.0 0.0 1.0 0.0 0.0 0.0 0.0 0.0
0.00585838    0.0 0.0 0.0 0.0 0.0 0.0 0.0 0.0 0.0 0.0 0.0 0.0 0.0 0.0 0.0 0.0 0.0 1.0 0.0 0.0 0.0 0.0
0.00334597    0.0 0.0 0.0 0.0 0.0 0.0 0.0 0.0 0.0 0.0 0.0 0.0 0.0 0.0 0.0 0.0 0.0 0.0 1.0 0.0 0.0 0.0
0.00204842    0.0 0.0 0.0 0.0 0.0 0.0 0.0 0.0 0.0 0.0 0.0 0.0 0.0 0.0 0.0 0.0 0.0 0.0 0.0 1.0 0.0 0.0
0.00132364    0.0 0.0 0.0 0.0 0.0 0.0 0.0 0.0 0.0 0.0 0.0 0.0 0.0 0.0 0.0 0.0 0.0 0.0 0.0 0.0 1.0 0.0
0.00089310    0.0 0.0 0.0 0.0 0.0 0.0 0.0 0.0 0.0 0.0 0.0 0.0 0.0 0.0 0.0 0.0 0.0 0.0 0.0 0.0 0.0 1.0
Ne P
234.94500      0.0018637129  -0.0002325222   0.0000107091  -0.0000429907   0.0003738603  -0.0003517440
55.077385      0.0144368802  -0.0017603337   0.0000805393  -0.0003240015   0.0028269923  -0.0026522743
17.389549      0.0655455723  -0.0081059303   0.0003802324  -0.0015003783   0.0129611220  -0.0121016505
6.3895370      0.1919505918  -0.0246273668   0.0011183944  -0.0045294322   0.0398964111  -0.0377131548
2.5420820      0.3493936429  -0.0492170997   0.0022603113  -0.0091034183   0.0822657993  -0.0793181401
1.0337640      0.3956032309  -0.0561815168   0.0025468717  -0.0101499112   0.0943376692  -0.0899698274
0.41878800     0.2047389632  -0.0310120557   0.0026180533  -0.0069506079   0.0290727168  -0.0138380624
0.16462700     0.0138949272   0.1023512480  -0.0123569722   0.0126714756  -0.3869789499   0.3837973808
0.05761900     0.0093620053   0.2505761725  -0.0284266987  -0.0301358904  -1.3945339063   1.3434793957
0.04233528    -0.0111611841   0.3042531367  -0.0657160178   0.2725443581   1.0754321215  -1.1958775614
0.01925421     0.0061177004   0.8724225945  -0.1531717163   0.5562091504   0.9401891546  -1.1295873123
0.00998821    -0.0071209447  -0.5528054898   0.4603629211  -1.5319718069  -0.4659020697   0.9925670366
0.00568936     0.0091045317  -0.1798678725   0.4759377271  -0.6216710256  -0.2232771060   1.3622486397
0.00347568    -0.0097318352  -0.1189668097   0.2570227575   1.2685463019   0.0562993054  -2.0141040571
0.00224206     0.0079224405   0.2686353415  -0.0323894548   0.5133406889  -0.6755011942  -0.0041620579
0.00151064    -0.0044646463  -0.0696963916   0.0317415552   0.2609943268  -0.1088498576  -0.6447441951
0.00105475     0.0012792313  -0.0212088242  -0.0088902706  -0.3425688911   1.2056376298   1.6972415185
Ne D
6.4200000      0.0002327144  -0.0015610076   0.0020109806
2.2470000      0.0007463332  -0.0045587641   0.0057582120
0.78645000     0.0034266133  -0.0259142298   0.0340449112
0.27525750     0.0042948074  -0.0367084557   0.0484963240
0.16329773     0.0193393737  -0.1898629249   0.2501956316
0.06054020     0.0900242792  -0.5043133352   0.5972605729
0.02744569     0.3346702372  -0.1128353381  -0.1792156753
0.01420440     0.4932777735   0.0939364131  -0.5887038263
0.00807659     0.1921250090   0.1193953290  -0.1703931380
0.00492719     0.0170430431   0.2603482660   0.4920300727
0.00317481    -0.0309291251   0.2717510449   0.3008438462
0.00213712    -0.0150705742   0.1298422386   0.2098560362
Ne F
4.1900000      0.0000241701  -0.0000391518
1.6760000      0.0001347578  -0.0002504648
0.67040000     0.0007803298  -0.0013482270
0.21400555     0.0120397134  -0.0225258780
0.07906987     0.0893736617  -0.1608630787
0.03576293     0.2555265976  -0.4315122957
0.01847779     0.3118937733  -0.3352314194
0.01049301     0.2113443838   0.1197315048
0.00639492     0.2217027219   0.4102217040
0.00411721     0.1142746337   0.2249266115
0.00276965     0.0983741234   0.1929267171
```

- QC III: (22s17p12d11f)/[9s8p5d4f]

Ne S

| | | | | | | | | | |
|---|---|---|---|---|---|---|---|---|---|
| 166165.08 | 0.0000 | -0.0000 | 0.0000 | -0.0000 | 0.0000 | -0.0000 | 0.0000 | 0.0000 | -0.0000 |
| 23107.524 | 0.0004 | -0.0001 | 0.0000 | -0.0000 | 0.0000 | -0.0000 | 0.0000 | 0.0000 | -0.0000 |
| 5060.1539 | 0.0022 | -0.0005 | 0.0001 | -0.0000 | 0.0000 | -0.0001 | 0.0001 | 0.0000 | -0.0000 |
| 1384.6123 | 0.0096 | -0.0024 | 0.0004 | -0.0001 | 0.0000 | -0.0004 | 0.0004 | 0.0000 | -0.0000 |
| 436.51258 | 0.0351 | -0.0089 | 0.0015 | -0.0004 | 0.0001 | -0.0015 | 0.0016 | 0.0001 | -0.0001 |
| 153.47148 | 0.1049 | -0.0277 | 0.0046 | -0.0012 | 0.0002 | -0.0047 | 0.0049 | 0.0003 | -0.0003 |
| 59.389087 | 0.2385 | -0.0693 | 0.0117 | -0.0031 | 0.0006 | -0.0120 | 0.0124 | 0.0009 | -0.0008 |
| 24.861967 | 0.3704 | -0.1311 | 0.0220 | -0.0057 | 0.0012 | -0.0222 | 0.0230 | 0.0016 | -0.0014 |
| 11.015704 | 0.3054 | -0.1662 | 0.0309 | -0.0082 | 0.0017 | -0.0325 | 0.0341 | 0.0024 | -0.0023 |
| 4.9651750 | 0.0832 | -0.0071 | 0.0015 | -0.0002 | 0.0000 | -0.0008 | 0.0021 | -0.0003 | 0.0005 |
| 1.9365030 | 0.0033 | 0.4415 | -0.0849 | 0.0220 | -0.0045 | 0.0894 | -0.0982 | -0.0058 | 0.0047 |
| 0.76572800 | 0.0007 | 0.5713 | -0.1913 | 0.0547 | -0.0118 | 0.2388 | -0.2584 | -0.0199 | 0.0193 |
| 0.29553800 | -0.0001 | 0.1218 | -0.1230 | 0.0394 | -0.0132 | 0.1114 | -0.0841 | -0.0056 | 0.0006 |
| 0.10343800 | 0.0002 | -0.0130 | 0.1017 | -0.0460 | 0.0066 | -0.7688 | 1.0169 | 0.0540 | -0.0178 |
| 0.06564559 | -0.0002 | 0.0089 | 0.3612 | -0.1964 | 0.0610 | -0.8099 | 0.6778 | 0.1659 | -0.2089 |
| 0.02462393 | 0.0001 | -0.0035 | 1.2334 | -0.8336 | 0.8883 | 1.8774 | -3.0894 | -0.4864 | 0.5907 |
| 0.01125334 | -0.0001 | 0.0036 | -0.6690 | 0.9454 | -1.8079 | -0.0414 | 1.6952 | -0.5593 | 0.0109 |
| 0.00585838 | 0.0002 | -0.0040 | -0.5411 | 0.9891 | -1.3819 | -0.9776 | 3.4980 | 3.7655 | -1.8740 |
| 0.00334597 | -0.0002 | 0.0044 | 0.6793 | -0.4056 | 2.9154 | 0.1501 | -5.6430 | -3.7723 | -2.7701 |
| 0.00204842 | 0.0002 | -0.0041 | -0.0644 | 0.1257 | -0.3728 | -1.7904 | 1.0781 | -1.8134 | 20.6876 |
| 0.00132364 | -0.0001 | 0.0023 | 0.0417 | -0.0656 | 0.2021 | 2.0906 | 0.9034 | 2.0417 | -30.2943 |
| 0.00089310 | 0.0000 | -0.0006 | -0.0258 | 0.0241 | -0.1583 | 0.1710 | 0.6692 | 1.1648 | 14.1291 |

Ne P

| | | | | | | | | |
|---|---|---|---|---|---|---|---|---|
| 234.94500 | 0.0018 | -0.0002 | 0.0000 | -0.0000 | 0.0004 | -0.0003 | 0.0000 | -0.0000 |
| 55.077385 | 0.0143 | -0.0017 | 0.0001 | -0.0003 | 0.0028 | -0.0026 | 0.0002 | -0.0002 |
| 17.389549 | 0.0653 | -0.0081 | 0.0004 | -0.0015 | 0.0129 | -0.0121 | 0.0007 | -0.0008 |
| 6.3895370 | 0.1918 | -0.0246 | 0.0011 | -0.0045 | 0.0398 | -0.0377 | 0.0022 | -0.0022 |
| 2.5420820 | 0.3494 | -0.0492 | 0.0022 | -0.0091 | 0.0823 | -0.0793 | 0.0042 | -0.0047 |
| 1.0337640 | 0.3958 | -0.0562 | 0.0025 | -0.0101 | 0.0943 | -0.0900 | 0.0051 | -0.0044 |
| 0.41878800 | 0.2048 | -0.0311 | 0.0026 | -0.0070 | 0.0292 | -0.0140 | 0.0031 | -0.0059 |
| 0.16462700 | 0.0139 | 0.1027 | -0.0123 | 0.0127 | -0.3868 | 0.3837 | -0.0293 | 0.0399 |
| 0.05761900 | 0.0095 | 0.2481 | -0.0285 | -0.0296 | -1.3944 | 1.3447 | -0.1268 | 0.0159 |
| 0.04233528 | -0.0113 | 0.3076 | -0.0647 | 0.2715 | 1.0749 | -1.1970 | 0.1017 | 0.1029 |
| 0.01925421 | 0.0063 | 0.8708 | -0.1525 | 0.5566 | 0.9404 | -1.1293 | 0.2895 | -0.7123 |
| 0.00998821 | -0.0075 | -0.5514 | 0.4601 | -1.5324 | -0.4657 | 0.9914 | -0.0079 | 1.3222 |
| 0.00568936 | 0.0095 | -0.1837 | 0.4750 | -0.6211 | -0.2237 | 1.3645 | -1.6572 | -2.1903 |
| 0.00347568 | -0.0102 | -0.1157 | 0.2575 | 1.2679 | 0.0567 | -2.0164 | 1.8177 | 8.9400 |
| 0.00224206 | 0.0083 | 0.2662 | -0.0324 | 0.5138 | -0.6760 | -0.0023 | 0.5743 | -23.9575 |
| 0.00151064 | -0.0047 | -0.0682 | 0.0319 | 0.2608 | -0.1087 | -0.6459 | 0.5885 | 28.5560 |
| 0.00105475 | 0.0013 | -0.0217 | -0.0090 | -0.3426 | 1.2059 | 1.6974 | -2.1804 | -12.3430 |

Ne D

| | | | | | |
|---|---|---|---|---|---|
| 6.4200000 | 0.0002 | -0.0016 | 0.0020 | 0.0004 | -0.0003 |
| 2.2470000 | 0.0007 | -0.0046 | 0.0058 | 0.0011 | -0.0009 |
| 0.78645000 | 0.0034 | -0.0260 | 0.0340 | 0.0061 | -0.0060 |
| 0.275257500 | 0.0042 | -0.0365 | 0.0489 | 0.0093 | -0.0043 |
| 0.16329773 | 0.0195 | -0.1902 | 0.2497 | 0.0419 | -0.0459 |
| 0.06054020 | 0.0894 | -0.5041 | 0.5975 | 0.1196 | -0.0823 |
| 0.02744569 | 0.3365 | -0.1129 | -0.1793 | -0.0300 | -0.0772 |
| 0.01420440 | 0.4900 | 0.0937 | -0.5889 | -0.3045 | 0.7403 |
| 0.00807659 | 0.1965 | 0.1198 | -0.1697 | -0.3555 | -0.9664 |
| 0.00492719 | 0.0129 | 0.2599 | 0.4914 | 0.4717 | 2.4093 |
| 0.00317481 | -0.0284 | 0.2720 | 0.3012 | 0.3991 | -5.7700 |
| 0.00213712 | -0.0158 | 0.1298 | 0.2098 | 0.4574 | 4.1147 |

Ne F

| | | | | |
|---|---|---|---|---|
| 4.1900000 | 0.0000 | -0.0000 | 0.0000 | -0.0000 |
| 1.6760000 | 0.0001 | -0.0002 | 0.0001 | 0.0001 |
| 0.67040000 | 0.0008 | -0.0014 | 0.0002 | -0.0008 |
| 0.21400555 | 0.0121 | -0.0225 | 0.0045 | -0.0021 |
| 0.07906987 | 0.0892 | -0.1611 | 0.0286 | -0.0487 |
| 0.03576293 | 0.2559 | -0.4308 | 0.1041 | -0.0358 |
| 0.01847779 | 0.3113 | -0.3363 | 0.1124 | -0.4500 |
| 0.01049301 | 0.2119 | 0.1208 | 0.1505 | 0.9052 |
| 0.00639492 | 0.2212 | 0.4092 | -0.4570 | -1.9310 |
| 0.00411721 | 0.1148 | 0.2259 | -0.0127 | 4.5540 |
| 0.00276965 | 0.0981 | 0.1924 | -0.7222 | -3.3404 |

[1] L. Avaldi, G. Dawber, R. Camilloni, G. C. King, M. Roper, M. R. F. Siggel, G. Stefani, M. Zitnik, A. Lisini, and P. Decleva, Phys. Rev. A **51**, 5025 (1995).

[2] A. Kivimäki, S. Heinäsmäki, M. Jurvansuu, S. Alitalo, E. Nõmmiste, H. Aksela, and S. Aksela, J. Electron Spectrosc. Relat. Phenom. **114**, 49 (2001).

[3] H. Yoshida, K. Ueda, N. M. Kabachnik, Y. Shimizu, Y. Senba, Y. Tamenori, H. Ohashi, I. Koyano, I. H. Suzuki, R. Hentges, J. Viefhaus, and U. Becker, J. Phys. B At. Mol. Opt. Phys. **33**, 4343 (2000).

[4] R. Manne and H. Ågren, Chem. Phys. **93**, 201 (1985).

[5] P.-O. Löwdin, Phys. Rev. **97**, 1474 (1955).
